# Supplementary material for: AugGen: Synthetic Augmentation using Diffusion Models Can Improve Recognition
Source: arXiv:2503.11544 source file (2025-10-24)
Supplement: Supplementary file 1 [file appendix.tex]

\section{Face Recognition Benchmarks}\label{app:exhaust_fr}
Here we present the same experiment setting as in \autoref{tab:challfr_benchmark} for IJB-B \cite{whitelam2017iarpaijbb} and IJB-C \cite{ijbc} for more thresholds set by usual False Positive Rates (FPRs), respectively presented in \autoref{tab:challfr_benchmark_ijbb} and \autoref{tab:challfr_benchmark_ijbc}.
We can observe again that our generated images consistently improve the discriminator trained on the original dataset in both the benchmarks and all the FPR values.

\begin{table*}[ht]
    \centering
    \caption{Comparison of the fully synthetic FR training, fully real FR training, and mixed FR training, when the models are evaluated against IJB-B with various FR thresholds. Here $n^{s}$ and $n^{r}$ depict the number of Synthetic and Real Images respectively and  Aux depicts whether the method for generating the dataset using an auxiliary information network for generating their datasets}
        \resizebox{\textwidth}{!}{ % This resizes the table to fit the page width
    
    \begin{tabular}{c||c|c|c||c|c|c|c|c|c||c}
        \toprule
        Method/Data & Aux & {$n^{s}$} & {$n^{r}$} & B-1e-6 & B-1e-5 & B-1e-4 & B-1e-3 & B-0.01 & B-0.1 & Avg \\
        \midrule
        DigiFace1M    &  N/A  & 1.22M & 0 & 15.31±0.42 & 29.59±0.82 & 43.53±0.77 & 59.89±0.51 & 76.62±0.44 & 91.01±0.12 & 52.66±0.47  \\
        RealDigiFace  &  \textcolor{red}{Y}  & 1.20M & 0 & 21.37±0.59 & 39.14±0.40 & 52.61±0.70 & 67.68±0.73 & 81.30±0.56 & 93.15±0.17 & 59.21±0.52  \\
        IDiff-face     &  \textcolor{red}{Y}  & 1.2M  & 0 & 26.84±2.03 & 50.08±0.48 & 64.58±0.32 & 77.19±0.41 & 88.27±0.15 & 95.94±0.05 & 67.15±0.50  \\
        DCFace        &  \textcolor{red}{Y}  & 0.5M  & 0 & 29.74±2.25 & 57.55±0.76 & 73.00±0.39 & 83.87±0.28 & 92.29±0.17 & 97.34±0.06 & 72.30±0.65  \\
        DCFace        &  \textcolor{red}{Y}   & 1.2M  & 0 & 22.48±4.35 & 47.84±6.10 & 73.20±2.53 & 86.11±0.59 & 93.55±0.16 & 97.56±0.06 & 70.12±2.28  \\
        Auggen, $\mathrm{D}^{\mathrm{aug}}$ (Ours)  &  \textcolor{teal}{N}  & $\sim$0.6M  & 0 & 32.67±1.17 & 51.52±0.69 & 67.77±0.83 & 80.24±0.50 & 90.30±0.03 & 96.74±0.03 & 69.87±0.52  \\
        Auggen $\mathrm{D}^{\mathrm{repro}}$ (Ours) &  \textcolor{teal}{N}  & $\sim$0.6M  & 0 & 15.71±3.12 & 45.97±4.64 & 73.05±0.89 & 85.54±0.16 & 93.52±0.17 & 97.82±0.08 & 68.60±1.43  \\

        \midrule
        \midrule 
        CASIA-WebFace  & N/A & 0     & $\sim$0.5M & 1.16±0.08 & 5.61±1.64 & 50.32±4.65 & 87.03±0.38 & 95.41±0.09 & 98.36±0.04 & 56.31±1.13  \\

        \midrule
        IDiff-face     & \textcolor{red}{Y} & 1.22M  & $\sim$0.5M  &  0.89±0.07 & 5.80±0.63 & 54.76±2.31 & 88.33±0.49 & 96.02±0.04 & 98.59±0.03 & 57.40±0.56  \\
        DCFace         & \textcolor{red}{Y} & 0.5M   & $\sim$0.5M  & 0.26±0.11 & 1.59±0.51 & 35.62±7.89 & 84.30±3.52 & 95.10±0.46 & 98.36±0.08 & 52.54±2.08  \\
        Auggen, $\mathrm{D}^{\mathrm{aug}}$  &  \textcolor{teal}{N} & $\sim$0.2M   & $\sim$0.5M  & 1.29±0.01 & 8.21±1.38 & 57.12±4.32 & 87.98±0.50 & 95.31±0.25 & 98.45±0.02 & 58.06±1.07  \\
        
        \bottomrule
    \end{tabular}
    }
    \label{tab:challfr_benchmark_ijbb}
\end{table*}

\begin{table*}[ht]
    \centering
    \caption{Comparison of the fully synthetic FR training, fully real FR training, and mixed FR training, when the models are evaluated against IJB-C with various FR thresholds. Here $n^{s}$ and $n^{r}$ depict the number of Synthetic and Real Images respectively and  Aux depicts whether the method for generating the dataset using an auxiliary information network for generating their datasets}
        \resizebox{\textwidth}{!}{ % This resizes the table to fit the page width
    
    \begin{tabular}{c||c|c|c||c|c|c|c|c|c||c}
        \toprule
        Method/Data & Aux & {$n^{s}$} & {$n^{r}$} & C-1e-6 & C-1e-5 & C-1e-4 & C-1e-3 & C-0.01 & C-0.1 & Avg \\
        \midrule
        DigiFace1M    &  N/A  & 1.22M & 0 & 26.06±0.77 & 36.34±0.89 & 49.98±0.55 & 65.17±0.39 & 80.21±0.22 & 92.44±0.05 & 58.37±0.46  \\
        RealDigiFace  &  \textcolor{red}{Y}  & 1.20M & 0 & 36.18±0.19 & 45.55±0.55 & 58.63±0.59 & 72.06±0.90 & 84.77±0.59 & 94.57±0.19 & 65.29±0.50  \\
        IDiff-face     &  \textcolor{red}{Y}  & 1.2M  & 0 & 41.75±1.04 & 51.93±0.89 & 65.01±0.63 & 78.25±0.39 & 89.41±0.19 & 96.55±0.05 & 70.48±0.47  \\
        DCFace        &  \textcolor{red}{Y}  & 0.5M  & 0 & 51.64±1.55 & 64.58±1.01 & 76.98±0.74 & 86.90±0.38 & 93.90±0.07 & 97.82±0.01 & 78.64±0.63  \\
        DCFace        &  \textcolor{red}{Y}   & 1.2M  & 0 & 35.27±10.78 & 58.22±7.50 & 77.51±2.89 & 88.86±0.69 & 94.81±0.09 & 98.06±0.06 & 75.46±3.65  \\
        Auggen, $\mathrm{D}^{\mathrm{aug}}$ (Ours)  &  \textcolor{teal}{N}  & $\sim$0.6M  & 0 & 47.74±0.47 & 58.07±0.48 & 71.61±0.50 & 82.87±0.32 & 92.03±0.04 & 97.37±0.04 & 74.95±0.31  \\
        Auggen $\mathrm{D}^{\mathrm{repro}}$ (Ours) &  \textcolor{teal}{N}  & $\sim$0.6M  & 0 & 31.54±6.65 & 58.61±3.89 & 78.11±0.51 & 88.51±0.04 & 94.79±0.09 & 98.17±0.04 & 74.96±1.82  \\    
        \midrule
        \midrule 
        CASIA-WebFace  & N/A & 0     & $\sim$0.5M & 0.83±0.10 & 5.86±1.31 & 56.87±3.14 & 89.41±0.40 & 96.19±0.06 & 98.61±0.02 & 57.96±0.83  \\

        \midrule
        IDiff-face     & \textcolor{red}{Y} & 1.22M  & $\sim$0.5M  &  0.70±0.11 & 7.46±2.08 & 57.43±4.17 & 89.89±0.71 & 96.63±0.08 & 98.77±0.01 & 58.48±1.19  \\
        DCFace         & \textcolor{red}{Y} & 0.5M   & $\sim$0.5M  & 0.18±0.07 & 1.54±0.59 & 38.17±8.24 & 86.18±3.32 & 95.88±0.42 & 98.59±0.05 & 53.42±2.11  \\
        Auggen, $\mathrm{D}^{\mathrm{aug}}$  &  \textcolor{teal}{N} & $\sim$0.2M   & $\sim$0.5M  & 1.43±0.22 & 9.67±1.01 & 61.75±3.48 & 90.00±0.44 & 96.17±0.19 & 98.64±0.01 & 59.61±0.81  \\
        
        \bottomrule
    \end{tabular}
    }
    \label{tab:challfr_benchmark_ijbc}
\end{table*}

\section{Experiment Details}\label{app:exp_details}
\subsection{Discriminator Training}
In the \autoref{tab:disc_training_params} the most important parameters for training our discriminative models are presented.

\subsection{Generator and Its Training}\label{app:generator}
We trained two sizes of generator namely small and medium as in \cite{Karras2024edm2}.
The training of the small-sized generator took about 1 NVIDIA H100 GPU day for the generator to see 805M images with a batch size of $2048$.
For reaching the same number of training images for the medium-sized generator, took about 2 days with a batch size of $1024$. 
We used an Exponential Moving Average (EMA) length of 10\%. As observed in literature \cite{nichol2021improved_ema}, the EMA of model weights plays a crucial role in the output quality of the Image Generators.

For sampling our models we did \textbf{not} employ any Classifier Free Guidance (CFG) \cite{ho2021classifierfree_cfg}.

\subsection{Table Details}
For the \autoref{tab:eff_auggen} we conditioned a medium-sized generator which trained till it saw 805M images. The conditions were set according to the four sets of values of the $\alpha$ and $\beta$. This is done for a fixed identity combination from the $\sL_{s}$ for all of them. Later for each of these new conditions $\vc^{*}$ we generated 50 images. 
All other tables were reported from a medium-sized generator when they saw 335M training samples.
%Results in the \autoref{tab:challfr_benchmark} and \autoref{}

\begin{table*}[ht]
    
    \centering
    \caption{Details of the Discriminator and its Training}
    \label{app:fr_dis_details}
    \resizebox{\textwidth}{!}{ % This resizes the table to fit the page width
    
    \begin{tabular}{c||c|c}
        \toprule
        Parameter Name & Discriminator Type 1 & Discriminator Type 2 \\ 
        \toprule
        Network type & ResNet 50  & ResNet 50                \\
        Marin Loss   & AdaFace    & AdaFace              \\
        \midrule 
        Batch Size & 192    & 512                   \\
        GPU Number & 4      & 1              \\
        Gradient Acc Step & 1 (For every training step )  & N/A             \\ 
        GPU Type   & Nvidia RTX 3090 Ti  & Nvidia H100             \\
        Precision of Floating Point Operations & High & High\\
        Matrix Multiplication Precision & High & High \\
        
        \midrule
        Optimizer Type & SGD & SGD  \\
        Momentum       & 0.9  & 0.9              \\
        Weight Decay   & 0.0005 & 0.0005             \\
        Learning Rate  & 0.1 & 0.1        \\
        WarmUp Epoch    & 1 & 1               \\
        Number of Epochs & 26 & 26                  \\
        LR Scheduler    & Step  & Step                \\
        LR Milestones   & $[12, 24, 26]$ & $[12, 24, 26]$      \\
        LR Lambda       & 0.1  & 0.1  \\
        \midrule
        Input Dimension & 112 $\times$ 112 & 112 $\times 112 $ \\
        Input Type      & RGB images & RGB Images         \\
        Output Dimension & 512 & 512             \\
        \midrule        
        Seed            & 41,2048,10 (In some models) & 41,2048                 \\
        \bottomrule
    \end{tabular}
    }
    \label{tab:disc_training_params}
\end{table*}

\section{Downstream Performance vs Metrics in Generative Models}\label{app:downstream_performance_vs_gen_metrics}
In this section, we examine whether there is a correlation between common metrics for evaluating generative models and the discriminator's performance when trained on our augmented dataset.
We studied the 
FD \cite{heusel2017gans}
Precision/Recall \cite{sajjadi2018assessing_precision,kynkaanniemi2019improved_recall_precision}
and 
Coverage \cite{naeem2020reliable_coverage} which is usually used to quantify the performance of the Generative Models. Calculation of these metrics requires the projection of the images into meaningful feature spaces. 
For feature extraction, we consider two backbones, Inception-V3 \cite{szegedy2016rethinking_inceptionv3} and DINOv2 \cite{oquab2023dinov2} which are shown effective for evaluating diffusion models \cite{stein2023exposing}. Both these models were trained using the ImageNet \cite{imagenet15russakovsky} in a supervised and semi-supervised manner respectively.
Experiments were performed by randomly selecting $100,000$ images of both CASIA-WebFace (as the source distribution) and our generated images by value of $\alpha$ and $\beta$ using \autoref{alg:grid_search} (\emph{i.e.}, the same settings as presented in the \autoref{sec:exps}). We are reporting four versions of our generated augmentation using a medium-sized generator when it sees 184M, 335M, 603M, and 805M training samples (M for Million). For each of the classes generated from these models we selected 20 samples, based on the observation in \autoref{tab:mixing_eff_chall}. Later by mixing the selected images with the original CASIA-WebFace we train FR for each of them and reporting the average accuracies for different thresholds in the IJB-C (\emph{i.e.}, similar to last column in the \autoref{tab:challfr_benchmark_ijbc}). \autoref{fig:aug_dinov2_vs_genmetrics} and \autoref{fig:aug_incv3_vs_genmetrics} are showing mentioned metrics for Inception-V3 and DINOv2 feature extractor respectively. 
We observe no clear correlation between the metrics used to evaluate generative models and the performance of a downstream task. This holds when we are augmenting the dataset for training the generator and discriminator with the original dataset. This highlights the need to develop new evaluation metrics.

\begin{figure}[htbp]
    \centering
    \begin{subfigure}[b]{0.24\textwidth}  % Adjust the width as needed
        \centering
        \includegraphics[width=\textwidth]{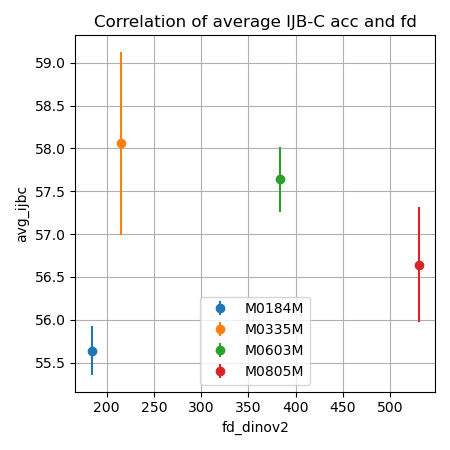}
        \caption{FD}
        \label{fig:dinov2_fd}
    \end{subfigure}
    \hfill
    \begin{subfigure}[b]{0.24\textwidth}
        \centering
        \includegraphics[width=\textwidth]{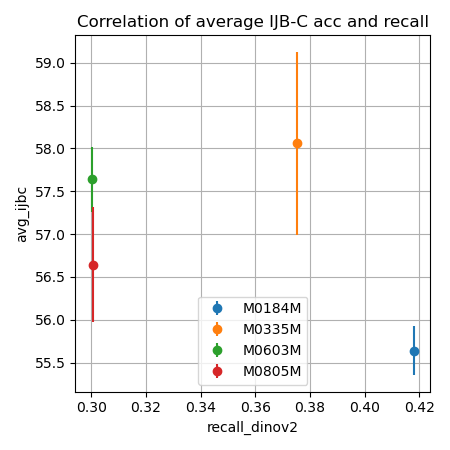}
        \caption{Recall}
        \label{fig:recall_dinov2}
    \end{subfigure}
    \hfill
    \begin{subfigure}[b]{0.24\textwidth}
        \centering
        \includegraphics[width=\textwidth]{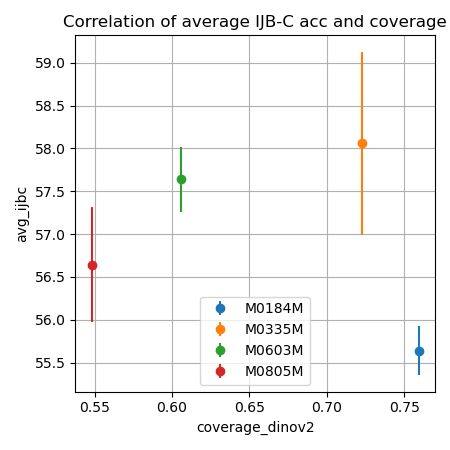}
        \caption{Coverage}
        \label{fig:cov_dinov2}
    \end{subfigure}
    \hfill
    \begin{subfigure}[b]{0.24\textwidth}
        \centering
        \includegraphics[width=\textwidth]{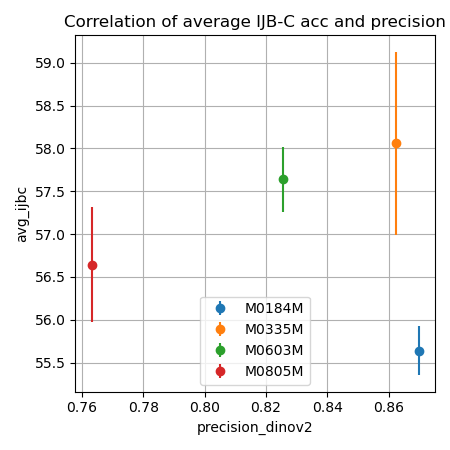}
        \caption{Precision}
        \label{fig:precision_dinov2}
    \end{subfigure}
    
    \caption{Correlation between the FD, Recall, Coverage, and Precision for the generated dataset by comparing it with the features of CASIA-WebFace using DINOv2 extractor.}
    \label{fig:aug_dinov2_vs_genmetrics}
\end{figure}

\begin{figure}[htbp]
    \centering
    \begin{subfigure}[b]{0.24\textwidth}  % Adjust the width as needed
        \centering
        \includegraphics[width=\textwidth]{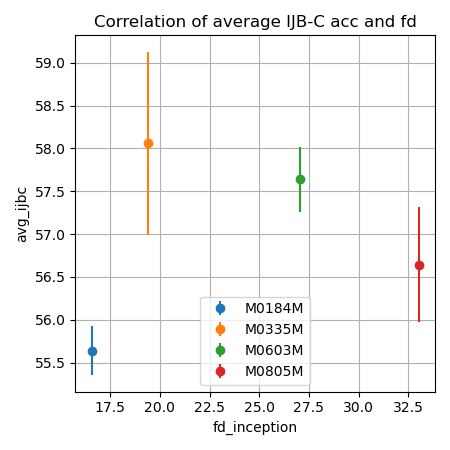}
        \caption{FD}
        \label{fig:fd_inc}
    \end{subfigure}
    \hfill
    \begin{subfigure}[b]{0.24\textwidth}
        \centering
        \includegraphics[width=\textwidth]{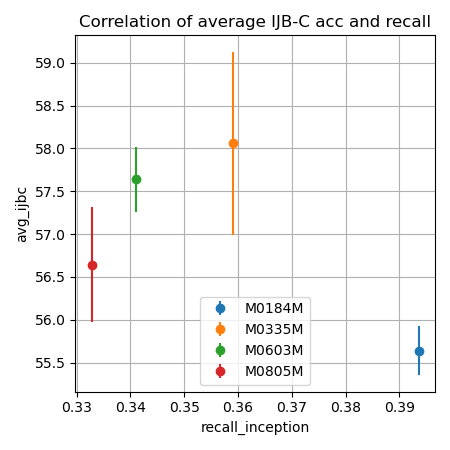}
        \caption{Recall}
        \label{fig:recall_inc}
    \end{subfigure}
    \hfill
    \begin{subfigure}[b]{0.24\textwidth}
        \centering
        \includegraphics[width=\textwidth]{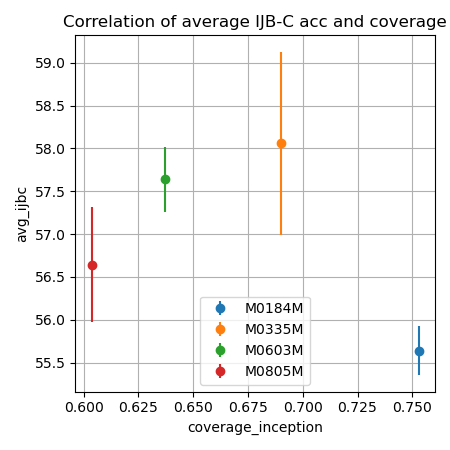}
        \caption{Coverage}
        \label{fig:cov_incp}
    \end{subfigure}
    \hfill
    \begin{subfigure}[b]{0.24\textwidth}
        \centering
        \includegraphics[width=\textwidth]{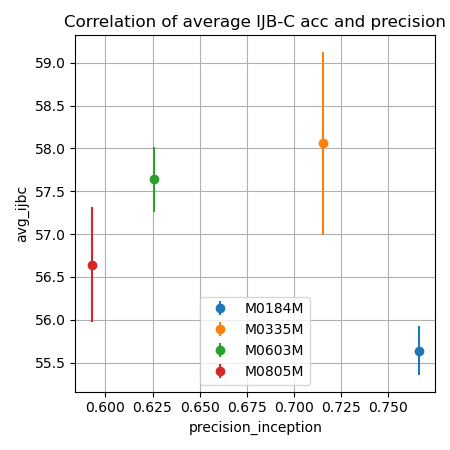}
        \caption{Precision}
        \label{fig:precision_incp}
    \end{subfigure}
    
    \caption{Correlation between the FD, Recall, Coverage, and Precision for the generated dataset by comparing it with the features of CASIA-WebFace using Inception-v3 extractor.}
    \label{fig:aug_incv3_vs_genmetrics}
\end{figure}

\section{Generated Images}\label{app:gen_imgs}
In the following figures, you can find more examples of generated images for Small and Medium-sized generators and also trained for more steps. By comparing \autoref{fig:sample_generated_app_s335k} (generated result from a small-sized generator trained when it sees 335M images, \textbf{S335M}), \autoref{fig:sample_generated_app_m335k} (\textbf{M335M}) and \autoref{fig:sample_generated_app_m805k} (\textbf{M805M}) we generally observe that larger generators are producing better images, but training for more steps does not necessarily translate to better image quality. 

\begin{figure}
    \centering
    \includegraphics[width=0.8\linewidth]{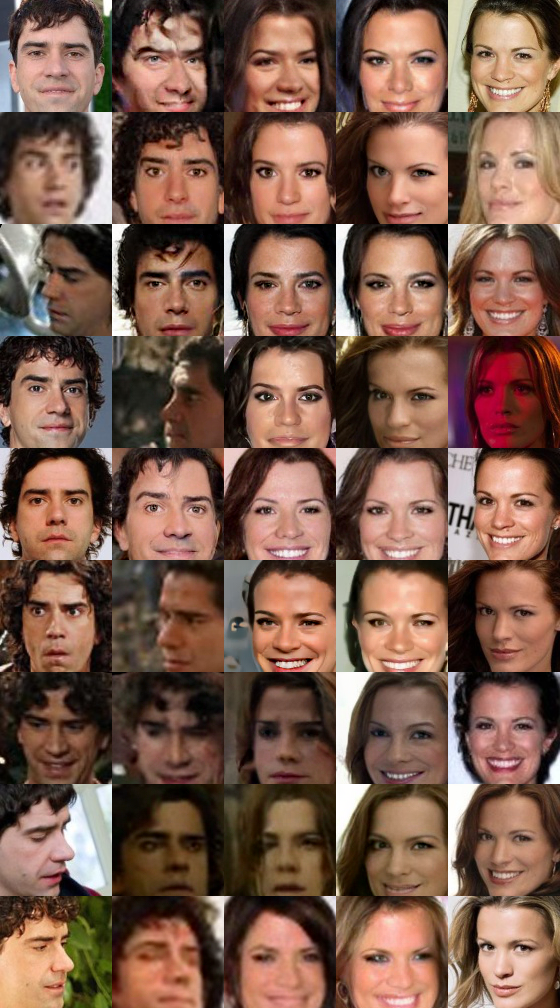} 
    \caption{Samll-sized generator trained till it sees 335M images. From left to right, the first column is variations of a random ID, 1, in the, $\mathrm{D}^\mathrm{orig}$, the second column is the recreation of the same ID in the first column using the generator when we put the conditions to 1, The last two columns are the same but for different IDs and the middle column representing the interpolated new identity.}
    \label{fig:sample_generated_app_s335k}
\end{figure}

\begin{figure}
    \centering
    \includegraphics[width=0.8\linewidth]{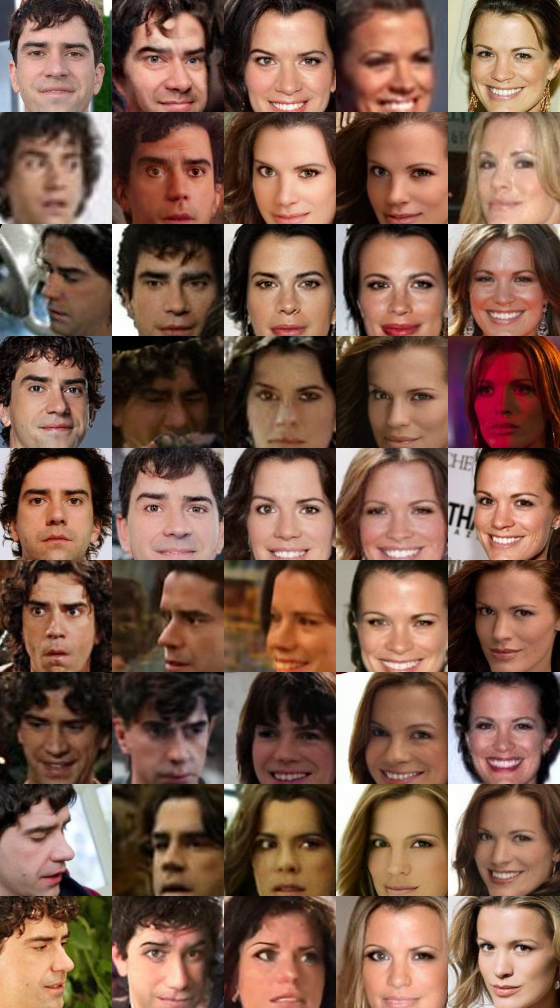} 
    \caption{Medium-sized generator trained till it sees 335M images. From left to right, the first column is variations of a random ID, 1, in the, $\mathrm{D}^\mathrm{orig}$, the second column is the recreation of the same ID in the first column using the generator when we put the conditions to 1, The last two columns are the same but for different IDs and the middle column representing the interpolated new identity.}
    \label{fig:sample_generated_app_m335k}
\end{figure}

\begin{figure}
    \centering
    \includegraphics[width=0.8\linewidth]{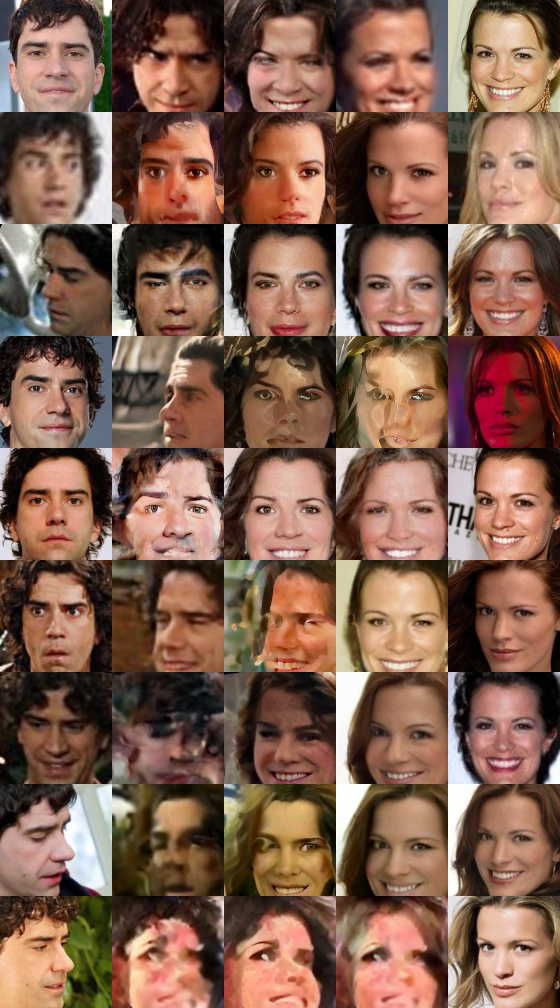} 
    \caption{Medium-sized generator trained till it sees 805M images. From left to right, the first column is variations of a random ID, 1, in the, $\mathrm{D}^\mathrm{orig}$, the second column is the recreation of the same ID in the first column using the generator when we put the conditions to 1, The last two columns are the same but for different IDs and the middle column representing the interpolated new identity.}
    \label{fig:sample_generated_app_m805k}
\end{figure}

\begin{figure}
    \centering
    \includegraphics[width=0.8\linewidth]{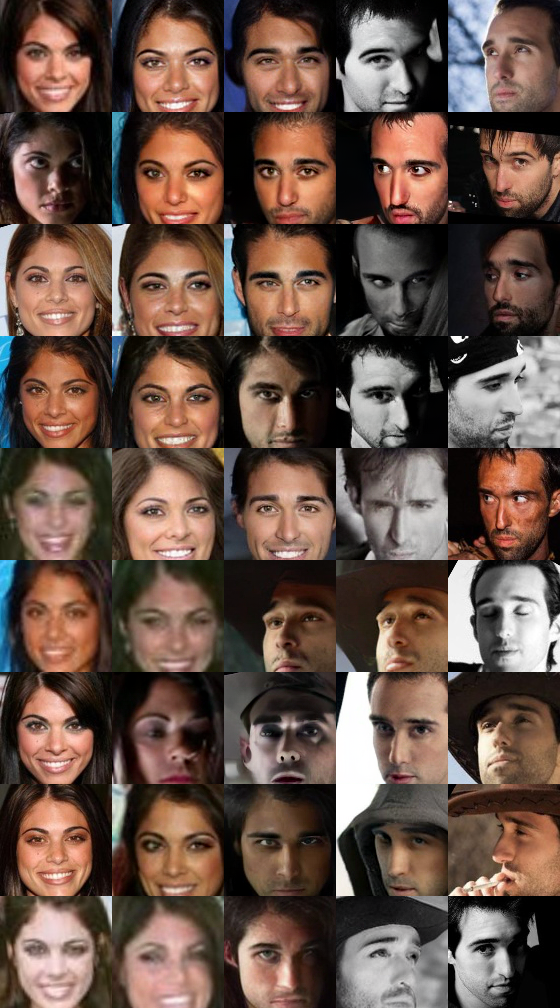} 
    \caption{Medium-sized generator trained for till it sees 335M images for different IDs. From left to right, the first column is variations of a random ID, 1, in the, $\mathrm{D}^\mathrm{orig}$, the second column is the recreation of the same ID in the first column using the generator when we put the conditions to 1, The last two columns are the same but for different IDs and the middle column representing the interpolated new identity.}
    \label{fig:sample2_generated_app_m335k}
\end{figure}

\section{Experiment Details}\label{app:exp_details}
\subsection{Discriminator Training}
In the \autoref{tab:disc_training_params} the most important parameters for training our discriminative models are presented.

\subsection{Generator and Its Training}\label{app:generator}
We trained two sizes of generator namely small and medium as in \cite{Karras2024edm2}.
The training of the small-sized generator took about 1 NVIDIA H100 GPU day for the generator to see 805M images with a batch size of $2048$.
For reaching the same number of training images for the medium-sized generator, took about 2 days with a batch size of $1024$. 
We used an Exponential Moving Average (EMA) length of 10\%. As observed in literature \cite{nichol2021improved_ema}, the EMA of model weights plays a crucial role in the output quality of the Image Generators.

For sampling our models we did \textbf{not} employ any Classifier Free Guidance (CFG) \cite{ho2021classifierfree_cfg}.

\subsection{Table Details}
For the \autoref{tab:eff_auggen} we conditioned a medium-sized generator which trained till it saw 805M images. The conditions were set according to the four sets of values of the $\alpha$ and $\beta$. This is done for a fixed identity combination from the $\sL_{s}$ for all of them. Later for each of these new conditions $\vc^{*}$ we generated 50 images. 
All other tables were reported from a medium-sized generator when they saw 335M training samples.
%Results in the \autoref{tab:challfr_benchmark} and \autoref{}

\begin{table*}[ht]
    
    \centering
    \caption{Details of the Discriminator and its Training}
    \label{app:fr_dis_details}
    \resizebox{\textwidth}{!}{ % This resizes the table to fit the page width
    
    \begin{tabular}{c||c|c}
        \toprule
        Parameter Name & Discriminator Type 1 & Discriminator Type 2 \\ 
        \toprule
        Network type & ResNet 50  & ResNet 50                \\
        Marin Loss   & AdaFace    & AdaFace              \\
        \midrule 
        Batch Size & 192    & 512                   \\
        GPU Number & 4      & 1              \\
        Gradient Acc Step & 1 (For every training step )  & N/A             \\ 
        GPU Type   & Nvidia RTX 3090 Ti  & Nvidia H100             \\
        Precision of Floating Point Operations & High & High\\
        Matrix Multiplication Precision & High & High \\
        
        \midrule
        Optimizer Type & SGD & SGD  \\
        Momentum       & 0.9  & 0.9              \\
        Weight Decay   & 0.0005 & 0.0005             \\
        Learning Rate  & 0.1 & 0.1        \\
        WarmUp Epoch    & 1 & 1               \\
        Number of Epochs & 26 & 26                  \\
        LR Scheduler    & Step  & Step                \\
        LR Milestones   & $[12, 24, 26]$ & $[12, 24, 26]$      \\
        LR Lambda       & 0.1  & 0.1  \\
        \midrule
        Input Dimension & 112 $\times$ 112 & 112 $\times 112 $ \\
        Input Type      & RGB images & RGB Images         \\
        Output Dimension & 512 & 512             \\
        \midrule        
        Seed            & 41,2048,10 (In some models) & 41,2048                 \\
        \bottomrule
    \end{tabular}
    }
    \label{tab:disc_training_params}
\end{table*}

\section{Generated Images}\label{app:gen_imgs}
In the following figures, you can find more examples of generated images for Small and Medium-sized generators and also trained for more steps. By comparing \autoref{fig:sample_generated_app_s335k} (generated result from a small-sized generator trained when it sees 335M images in different noise levels when optimizing the score-function using \autoref{eq:den_stage_2}, \textbf{S335M}), \autoref{fig:sample_generated_app_m335k} (\textbf{M335M}) and \autoref{fig:sample_generated_app_m805k} (\textbf{M805M}) we generally observe that larger generators are producing better images, but training for more steps does not necessarily translate to better image quality. 

\begin{figure}
    \centering
    \includegraphics[width=0.8\linewidth]{sec/imgs/mixes_imgs/mixed_test_3211-6825_half++.png} 
    \caption{Samll-sized generator trained till it sees 335M images. From left to right, the first column is variations of a random ID, 1, in the, $\mathrm{D}^\mathrm{orig}$, the second column is the recreation of the same ID in the first column using the generator when we put the conditions to 1, The last two columns are the same but for different IDs and the middle column representing the interpolated new identity.}
    \label{fig:sample_generated_app_s335k}
\end{figure}

\begin{figure}
    \centering
    \includegraphics[width=0.8\linewidth]{sec/imgs/mixes_imgs/edm2-m-335k-half++_mixed_test_3211-6825.png} 
    \caption{Medium-sized generator trained till it sees 335M images. From left to right, the first column is variations of a random ID, 1, in the, $\mathrm{D}^\mathrm{orig}$, the second column is the recreation of the same ID in the first column using the generator when we put the conditions to 1, The last two columns are the same but for different IDs and the middle column representing the interpolated new identity.}
    \label{fig:sample_generated_app_m335k}
\end{figure}

\begin{figure}
    \centering
    \includegraphics[width=0.8\linewidth]{sec/imgs/mixes_imgs/edm2-m-805k-full_mixed_test_3211-6825.png} 
    \caption{Medium-sized generator trained till it sees 805M images. From left to right, the first column is variations of a random ID, 1, in the, $\mathrm{D}^\mathrm{orig}$, the second column is the recreation of the same ID in the first column using the generator when we put the conditions to 1, The last two columns are the same but for different IDs and the middle column representing the interpolated new identity.}
    \label{fig:sample_generated_app_m805k}
\end{figure}

\begin{figure}
    \centering
    \includegraphics[width=0.8\linewidth]{sec/imgs/mixes_imgs/edm2-m-335k-half++_mixed_test_425-88.png} 
    \caption{Medium-sized generator trained for till it sees 335M images for different IDs. From left to right, the first column is variations of a random ID, 1, in the, $\mathrm{D}^\mathrm{orig}$, the second column is the recreation of the same ID in the first column using the generator when we put the conditions to 1, The last two columns are the same but for different IDs and the middle column representing the interpolated new identity.}
    \label{fig:sample2_generated_app_m335k}
\end{figure}

% \begin{figure}
%     \centering
%     \includegraphics[width=0.8\linewidth]{sec/imgs/mixes_imgs/mixed_test_1935-8643_half++.png} 
%     \caption{From left to right, the first column is variations of a random ID, 1, in the, $\mathrm{D}^\mathrm{orig}$, the second column is the recreation of the same ID in the first column using the generator when we put the conditions to 1, The last two columns are the same but for different IDs and the middle column representing the interpolated new identity.}
%     \label{fig:sample_generated}
% \end{figure}
